# Supplementary material for: Adaptive Sample Sharing for Multi Agent Linear Bandits
Source: arXiv:2309.08710 source file (2025-05-27)
Supplement: Supplementary file 1 [file table_R_T_8_supp_benchmark_synth.tex]

\scalebox{0.8}{% 
\hspace*{-0.55cm} 
\begin{tabular}{l|cc} 
   \textbf{Cumul. regret} & $M = N = 100$ \\ 
    \midrule 
    Ind & \textbf{4543.0 +/- 353.8} \\ 
    \emph{Oracle} & 4400.5 +/- 344.2 \\ 
    DynUCB & 92224.8 +/- 6743.8 \\ 
    CLUB ($\gamma=\Delta^{\min}_{\bm{\theta}, 2}/4$) & 5918.0 +/- 621.3 \\ 
    CLUB ($\gamma=\Delta^{\min}_{\bm{\theta}, 2}/2$) & 8627.9 +/- 1901.7 \\ 
    SCLUB ($\gamma=\Delta^{\min}_{\bm{\theta}, 2}/4$) & 4768.1 +/- 385.6 \\ 
    SCLUB ($\gamma=\Delta^{\min}_{\bm{\theta}, 2}/2$) & 4716.2 +/- 442.3 \\ 
    BASS ($\delta=0.1$) & 12411.4 +/- 7191.2 \\ 
    BASS ($\delta=0.9$) & 12277.7 +/- 3595.3 \\ 
    CMLB ($\gamma=\Delta^{\min}_{\bm{\theta}, 2}/4$) & 8470.9 +/- 20939.3 \\ 
    CMLB ($\gamma=\Delta^{\min}_{\bm{\theta}, 2}/2$) & 5849.1 +/- 65748.3
\end{tabular} 
}
